# Supplementary material for: Dexterous In-hand Manipulation by Guiding Exploration with Simple Sub-skill Controllers
Source: arXiv:2303.03533 source file (2023-09-26)
Supplement: Supplementary file 1 [file appendix.tex]

% We select a finger with an index $i$, initialize a switching step $t_s=0$ ($t_s=0$ indicates the finger is not in a switching process, otherwise it is.) to record how many step the finger has been switching. Each step if $t_s = 0$ we make $t_s = 1$ so it is in the switching process, and randomly select a rotation velocity $\omega_2$. Else when $t_s > 0$, $t_s$ increment by 1 each step and move the fingertip away from the object, rotate with $\omega_2$ and then move back approaching the object. We use a contact ensure factor $a$ slightly smaller than 0.5 to make approaching longer than leaving the object so the finger is more likely to remake contact. Fingers are moved by simply control the position change of proximal joint $q_p(t_s)$ and middle joint $q_m(t_s)$.
% \begin{algorithm}
% \caption{Joint trajectory Joint trajectory for contact switching}
% \begin{algorithmic}[1]
% \State \textbf{Input:} Finger index $i$, contact ensure factor $a \in{0<a<0.5}$, detaching and approaching angular velocity $\omega_1$, mean and std finger rotation velocity $\bar{\omega_2},\sigma$, expected switching time $T$, switching step $t_s=0$, 
% \Repeat
% \State Initialize change of proximal joint position and middle joint position $q_p=0$ and $q_m=0$.
% \If{$t_s = 0$}
% \State Set $t_s=1$ to start switching process.
% \State Randomly sample a finger rotation velocity $\omega_2$ %$\sim N(\bar{\omega_2},\sigma)$.
% \Else
% \If{$F(i)$ in contact with object \textbf{and} $t_s > T/2$} 
% \State $t_s=0$
% \Else
% \If{$t_s < 0.5T$} 
% \State $\dot{q}_m=\omega_1$ to move middle joint outward
% \State $t_s += 1$
% \ElsIf{$0.5T \leq t_s < aT$}
% \State $\dot{q}_m=\omega_1$ to move middle joint outward
% \State $\dot{q}_p=\omega_2$ to move proximal joint
% \State $t_s += 1$
% \ElsIf{$aT \leq t_s < 1.5T$}
% \State $\dot{q}_m=-\omega_1$ to move middle joint inward
% \State $\dot{q}_p=\omega_2$ to move proximal joint
% \State $t_s += 1$
% \ElsIf{$1.5T \leq t_s < 2T$}
% \State $\dot{q}_m=-\omega_1$ to move middle joint inward
% \State $t_s += 1$
% \Else
% \State $t_s=0$ to stop rotation process
% \EndIf
% \EndIf
% \end{algorithmic}
% \label{algo:sf_switch_expert}
% \end{algorithm}
